# Supplementary material for: Deep End-to-End Survival Analysis with Temporal Consistency
Source: arXiv:2410.06786 source file (2026-10-09)
Supplement: Supplementary file 1 [file tcsr_desc.tex]

Algorithm~\ref{alg:tcsr} describes the TCSR method by \cite{TemporallyConsistentSA}. 
After obtaining the soft targets and weights in lines 3 to 11 for the whole dataset, the objective in line 14 is optimized to update the model's parameters.
In Table~\ref{tab:comparsion_algs} in Appendix~\ref{appendix:comparison} we summarize the main hyperparameters for the benchmark survival algorithm with and without landmarking, for TCSR and our method, DeepTCSR.
\vspace{-0.2cm}
\begin{algorithm}
\caption{TCSR($\lambda$).}
\label{alg:tcsr}
\textbf{Inputs:} Sequences $\{(x_{m0}, \ldots, x_{mt_m})\}$, initial parameters $\theta$, decay $\lambda \in [0, 1]$
\begin{algorithmic}[1]
\REPEAT
    \FOR{$\ell = 1, \ldots, K$} %\COMMENT{Weights and targets for $\ell$-step lookahead.}
        \FOR{$m = 1, \ldots, M$}
            \FOR{$k = 1, \ldots, \ell$} %\COMMENT{Based on observed outcomes.}
                \STATE $y^{(\ell)}_{mk} \gets 1\{t_m = k \land x_{t_m} = \emptyset\}$
                \STATE $w^{(\ell)}_{mk} \gets 1\{t_m \geq k\}$
            \ENDFOR
            \FOR{$k = \ell + 1, \ldots, K$} %\COMMENT{Based on predictions at $x_{\ell}$.}
                \STATE $y^{(\ell)}_{mk} \gets h_{\theta}(k - \ell | x_{m\ell})$
                \STATE $w^{(\ell)}_{mk} \gets S_{\theta}(k - \ell - 1 | x_{m\ell})$
            \ENDFOR
        \ENDFOR
        \STATE $c_{\ell} \gets (1 - \lambda) 1^{\{\ell < K\}}\lambda^{\ell}$
        \STATE $\theta \gets \arg\min_{\theta} \sum_{\ell=1}^{K} c_{\ell} \sum_{m=1}^{M} \sum_{k=1}^{K} w^{(\ell)}_{mk} H\left[y^{(\ell)}_{mk} \| h_{\theta}(k | x_{m})\right]$
    \ENDFOR
\UNTIL $\theta$ has converged
\end{algorithmic}
\end{algorithm}
